# Supplementary material for: 3D Scene Inference from Transient Histograms
Source: arXiv:2211.05094 source file (2022-11-09)
Supplement: Supplementary file 1 [file supplement.tex]

%\documentclass{article}
%\usepackage[utf8]{inputenc}
%\usepackage{graphicx} % For adding figs
%\usepackage{amssymb} % For not exists, etc..
%\usepackage{amsfonts} % For real nums, integers sets, etc..
%\usepackage{amsmath} % For equations, etc...
%\usepackage{mathtools}
%\usepackage{float}

%\usepackage[margin=0.8in]{geometry}
%\usepackage{siunitx}  % For margins

%\title{Supplemental Document}
%\author{Sacha Jungerman, Atul Ingle, Yin Li, Mohit Gupta\\
%University of Wisconsin-Madison\\
%{\tt\small \{sjungerman, ingle, yin.li, mgupta37\}@wisc.edu}}
%\author{Anonymous CVPR Submission}
%\begin{document}
%\maketitle

%\captionsetup[figure]{name={Suppl. Fig.}}

\setcounter{figure}{0}
\setcounter{section}{0}
\setcounter{equation}{0}
\setcounter{page}{1}

\begin{center}
%\begin{tabular}{c}
\huge Supplementary Document for\\
\huge ``3D Scene Inference from Transient Histograms'' \\[0.2in]
\large Sacha Jungerman, Atul Ingle, Yin Li, Mohit Gupta\\
University of Wisconsin-Madison\\
{\tt\small \{sjungerman, ingle, yin.li, mgupta37\}@wisc.edu}
\end{center}

\section{Inference from Scenes with Non-Uniform Albedos}

\begin{figure}[!ht]
\centering \includegraphics[width=0.9\textwidth]{figures/albedo-or-no.pdf}
\caption{\textbf{Robustness to Albedo Variations.} We again show a few NYUv2 patches and their accompanying transients. We show the transients the AbS method has fitted to when not estimating scene albedo (a) and when jointly estimating scene albedo (b).
%Finally, the color bar below each transient shows the average albedo per bin. Their homogeneity largely causes the observed robustness to albedo variations.
\label{fig:albedo-vars}}
\end{figure}

%\smallskip
\noindent \textbf{Robustness to albedo variations:} We observe that, in most cases, both the theoretical and AbS approaches are robust to real-world albedo variations, and slight geometry variations, despite making no explicit attempt at modeling non-uniform albedos. This is seen in both sample scenes in Suppl. Fig.~\ref{fig:albedo-vars}(a): the dashed transient are nearly identical which indicates good parameter estimation despite challenging albedo variations.

We attribute this robustness to albedo variations to the implicit albedo averaging that is performed through binning. Each transient bin will receive contributions from all scene patches at a specific distance from the sensor. The perceived albedo at that bin will thus effectively be the average albedo of all those scene patches. This is illustrated in Suppl. Fig.~\ref{fig:albedo-vars}(a) as the horizontal greyscale color bar under each transient. While this per-bin albedo average could have sharp transitions for a carefully crafted, adversarial scene, we observe that when imaging real scenes, albedos are smooth over consecutive bins.

\smallskip
\noindent \textbf{Estimating scene albedo:}
We can try to recover the scene's point-wise albedo by augmenting our AbS approach with a texture that stores the scene's albedo. Gradients with respect to this texture can then be computed, and the texture optimized. However, due to the albedo binning process described above, the best we can aim to recover is the average albedo per bin. The optimized albedo-texture cannot contain the scene's albedo as a single transient does not contain enough spatial information.

With no added regularization, the albedo-texture map converges to what looks like salt and pepper noise. While this albedo map is of no immediate use, it can help the AbS method converge to better plane estimates. In Suppl. Fig.~\ref{fig:albedo-vars}(b) we show sample results for which the scene's albedo was estimated. Notice that when jointly estimating plane parameters and albedo, the AbS transient (green) can more closely fit the observed one (blue). As seen in the last row, this can cause over-fitting issues and lead to estimated parameters that describe a plane that best fits the observed geometry instead of the planar part of the scene.

%While both the theoretical approach and the AbS approach make no explicit attempt to model non-uniform albedoes, we observe that in practice, both are robust to real-world albedo variations. Fig.~\ref{fig:albedo-vars} shows examples of this albedo invariance.

%%\textcolor{orange}{
%%    TODO: Discuss whether it makes sense to try to recover albedos if we should regress over albedos when performing AbS and the differences that makes.
%%}
%
%\smallskip
%\noindent \textbf{Robustness to geometry variations:}
%Despite only modeling perfectly planar scenes in our models, real scenes are often more complex, cluttered, and do not satisfy this assumption. We observe in practice that when the scene is mostly planar our method still produces reliable plane estimates.
%
%In the third row for figure~\ref{fig:robustness}, the patch is not quite planar as the gym equipment clutters the view. Notice that the RANSAC estimate fits to the biggest transient spike whereas the AbS method tries to minimize the error over the whole transient. This behavior could be used to distinguish mostly-planar scene patches from non-planar patches: if the estimates from the theoretical approach and AbS approach are different enough, we characterize the patch as non-planar.
%% TODO: Not sure the above makes sense, we don't show the theoretical estimate in figure~\ref{fig:robustness}, and even if we did, the transient has two peaks, no need for fancy methods, it's non-planar.

\newpage
\section{Deep Model and Training Details}

\smallskip
\noindent\textbf{Model Architecture:}

\begin{figure}[!h]
\centering \includegraphics[width=0.8\textwidth]{figures/architecture.pdf}
\caption{\textbf{Architecture of Model.} Diagram showing our model architecture and the refinement steps. We use two existing methods~\cite{kim_deformable_2021,ranftl_vision_2021} (seen in blue) to refine our depth predictions. \label{fig:architecture}}
\end{figure}

Suppl. Fig.~\ref{fig:architecture} shows the full architecture of our model and the refinement steps. Transients are first encoded as their first $k$ Fourier coefficients and then passed to our base network which consists of a few blocks, each containing two convolutions followed by bilinear upsampling by a factor of $2\times$. For the $20\times15$ tiling, we use $k=16$ and five blocks. For the $4\times3$ tiling, which is $160\times$ smaller than the output dimension, we use six blocks with the first one upsampling by a factor of $5\times$, and we use $k=4$.

The refinement step consists of two off-the-shelf networks: DKN~\cite{kim_deformable_2021} and DPT~\cite{ranftl_vision_2021}. The former was finetuned to refine our depth estimate using the RGB image as an added input, while the latter is pretrained and only uses the RGB image. We then use the depth map produced by DKN as a guide to warp the DPT depth map. We first tile each depth map, then compute the scale and shift that will minimize the $\mathcal{L}_2$ loss between them. This scale and shift tensor, of shape $n \times m \times 2$, is then bilinearly interpolated to the full resolution of $640\times480$ and applied to DPT's output. This enables our approach to gain from the spatial details present in DPT's output but not suffer from its low accuracy. The tiling grid used by the tile-wise matching process can be adjusted to yield results with greater details or greater accuracy. For our experiments, it matched the transient tiling grid.

\smallskip
\noindent\textbf{Loss Function}:
Traditionally, the loss function used for regression problems is the squared Euclidean distance, or the $\mathcal{L}_2$ norm $\mathcal{L}_2(\tilde{y} - y) = ||\tilde{y} - y||_2^2$ between the predictions $\tilde{y}$ and ground truth $y$.  However,
using this simple $\mathcal{L}_2$ loss function leads to blurry depth reconstructions \cite{laina_deeper_2016,godard_unsupervised_2017,kuznietsov_semi-supervised_2017}. To alleviate this, we use the reverse Hubert loss (a.k.a: BerHu loss), $\mathcal{B}$, as introduced by~\cite{verducci_robust_2007,zwald_berhu_2012}.

\begin{equation}
    \mathcal{B}(x) =
        \begin{cases}\label{eq:berhu}
            |x| & |x| \leq c, \\
            \frac{x^2 + c^2}{2c} & |x| > c. \\
        \end{cases}
\end{equation}

This loss effectively acts like an $\mathcal{L}_1$ loss for small errors and an $\mathcal{L}_2$ for large ones. It has the advantage of penalizing large errors as much as an $\mathcal{L}_2$ loss would while still providing a large enough gradient for smaller errors.
%TODO [insert sparsity argument of L1 / L2?].
This yields a sharper final prediction and a lower final error. Further, the hyper-parameter $c$ can be used to tune the BerHu loss and change where the $\mathcal{L}_1$/$\mathcal{L}_2$ switch occurs.\\

\smallskip
\noindent\textbf{Implementation details:}
Unless otherwise noted, all experiments used a BerHu loss with tuning parameter $c=0.1$ and ran on a single GeForce RTX 3090 or a GeForce RTX 2080 Super for up to $500$ epochs. We used the Adam optimizer, with a learning rate of $0.01$.
%and a learning weight scheduler decay of $0.8$ per epoch.
Transient histograms are simulated from the ground-truth data using Eq.~(\ref{eq:signalflux}) where we used the green channel of the RGB images as a proxy for scene albedoes.

\newpage
\section{Definition of Metrics Used}

The metrics used to evaluate our results follow that of previous work~\cite{eigen_depth_2014} and are defined as follows:

\begin{itemize}
    \item Absolute Relative Error (AbsRel):
        \begin{align*}
            \frac{1}{n}\Sigma_{n} \frac{\lvert\hat{y}_i - y_i\rvert}{y_i}
        \end{align*}\label{eq:abs_rel}
    \item Root Mean Squared Error (RMSE):
        \begin{align*}
            \sqrt{\frac{1}{n}\Sigma_{n} \lVert{\hat{y}_i - y_i}\rVert_2}
        \end{align*}\label{eq:rmse}
    \item Average Log Error (Log10):
        \begin{align*}
            \frac{1}{n}\Sigma_{n} \lvert{log_{10}(\hat{y}_i) - log_{10}(y_i)}\rvert
        \end{align*}\label{eq:log10}
    \item Threshold Accuracy ($\delta < thr$):
        \begin{align*}
            \max\left(\frac{\hat{y}_i}{y_i},  \frac{y_i}{\hat{y}_i}\right) = \delta < thr
        \end{align*}\label{eq:thr_acc}
\end{itemize}
where $\hat{y}_i$ is a pixel in the predicted depth map $\hat{y}$, $y_i$ is a pixel in the ground-truth depth map $y$, and $n$ is the number of valid pixels. Again, prior work has only used $1.25^i$ for $i = 1,2,3$ as the threshold for the threshold accuracy metric. These correspond to $25\%$, $56\%$, and $95\%$ error respectively. We have introduced the tighter thresholds of $1.05^i$ for $i=1,2,3$ to better characterize approaches. These correspond roughly to $5\%$, $10.25\%$, and $15.76\%$ error.

%TODO: Add an accuracy curve/Show one for hardware results #2? Add plot showing MSE error of DPT for low metrics?

\newpage
\section{Comparison with MDE}

\begin{figure}[!h]
\centering \includegraphics[width=0.9\textwidth]{figures/mde-error-supp.pdf}
\caption{\textbf{Results and $\mathcal{L}_1$ Error on NYUv2 Dataset.} From left to right this figure shows the RGB image, ground truth depth, our refined for the $20\times15$ grid, the absolute error of our approach, a MDE result from DPT~\cite{ranftl_vision_2021}, and their absolute error. \label{fig:mde-error}}
\end{figure}

In Suppl. Fig.~\ref{fig:mde-error}, we show results from our method and a leading MDE method. While visually DPT results look marginally better, they often have large absolute depth errors. Even for small indoor scenes of less than 10 meters, DPT can produce absolute errors of the order of 2 meters. For these reasons our method is better suited for applications that require precise depth.

\newpage
\section{Additional Hardware Results}

While our hardware setup, shown in Fig.~\nolink{\ref{fig:lab-setup-results}}(left), has a bin-width of \SI{16}{\pico\second}, our models were trained with transients having 512 bins over an unambiguous depth of \SI{10}{\meter}. Instead of retraining our models, we preprocess the measured transients by re-binning them accordingly and subsequently applying a small amount of Gaussian smoothing ($\sigma=2$ bins).

\begin{figure}[!h]
\centering \includegraphics[width=0.9\textwidth]{figures/real-transients.pdf}
\caption{\textbf{Transient Histogram Preprocessing.} We show example measured, simulated and processed transients. \label{fig:real-transients}}
\end{figure}

An assumption which was made while training the network on simulated data is that the laser pulse could be modeled as a Dirac delta pulse (with respect to the bin-width), however, the hardware setup uses a laser with a pulse width of \SI{6}{\nano\second} which corresponds to about $375$ bins. Not only is the pulse width much larger than in simulation, but it is also not the same shape: all measured transients are effectively convolved with an unknown kernel.

To estimate this kernel, we first simulated transients from the ground truth depth, as measured by the Kinect, using a laser pulse of larger width. We then trained a shallow fully connected neural network to map the measured transients to the simulated ones using only $20\%$ of the acquired data as a training set. This small model was trained with an Adam optimizer (with default parameters) and a Kullback-Leibler divergence loss. Examples of the measured transients, simulated ones, and neural network processed ones are shown in Suppl. Fig.~\ref{fig:real-transients}.

\begin{figure}[!h]
\centering \includegraphics[width=0.7\textwidth]{figures/hardware-results-supp.pdf}
\caption{\textbf{Results with experimental setup.} (a) We image a table-top scene with a wide range of albedos and textured objects. (b) The true depth map captured using a Kinect v2. (c) Since the capture is a low-resolution $20\times 15$ grid, simple peak-finding-based depth map provides no depth details. (d) Using the RGB image as a guide, our method generates a high-resolution depth map. \label{fig:hardware-results-supp}}
\end{figure}

\begin{figure}[!h]
\centering \includegraphics[width=0.7\textwidth]{figures/accuracy-curve.pdf}
\caption{\textbf{Threshold Accuracy on Real Data.} We show the continuous threshold accuracy for our method without refinement (``Base''), with refinement (``Refined''), and DPT~\cite{ranftl_vision_2021} for all thresholds in the range $[1, 2]$. Results are reported on a single scene in Suppl.~Fig.\ \ref{fig:hardware-results-supp}. %Notice that our method performs better overall, and especially for lower thresholds.
\label{fig:accuracy}}
\end{figure}

Results using the processed transients can be seen in Fig.~\nolink{\ref{fig:lab-setup-results}}(right) and Suppl. Fig.~\ref{fig:hardware-results-supp}. Finally Suppl. Fig.~\ref{fig:accuracy} shows the accuracy of our method (with and without refinement) as well as DPT's~\cite{ranftl_vision_2021} on the scene shown in Suppl. Fig.~\ref{fig:hardware-results-supp}. Our results, on this scene, achieve better threshold accuracy overall, especially for lower thresholds. With more data this preprocessing scheme would not be needed, as our model could be finetuned to adapt to the characteristics of the hardware setup in use.

\clearpage
\section{Dealing with Pile-up Distortions}

\begin{figure}[!h]
\centering \includegraphics[width=0.9\textwidth]{figures/spad_measure_th.pdf}
\caption{\textbf{Measuring a transient histogram using a SPAD.} (a) The test scene consists of
a ring-shaped target with a background wall. (b) Asynchronous acquisition using
a SPAD reliably captures later photons by avoiding pile-up distortion seen in
conventional acquisition.\label{fig:spad_th_measure}}
\end{figure}

If the total photon flux incident on the SPAD is high enough, photon detections in earlier histogram bins prevent later bins from capturing photons. This causes pile-up distortions that follow a characteristic exponentially decaying shape. This pile-up can be due to ambient light or due to laser photons reflecting from a high albedo target. Suppl. Fig.~\ref{fig:spad_th_measure} shows a histogram with and without pileup for the ring-shaped target with a wall in the background. Observe that the pile-up distorted histogram has fewer total photon counts in later photon bins. We use an \emph{asynchronous} acquisition scheme~\cite{gupta_asynchronous_2019} that counteracts pile-up distortion by operating the SPAD in a free-running mode. The SPAD pixel enters a dead-time immediately after each photon detection event and is reset to capture the next photon after the dead-time period ends. By capturing raw timestamps for each photon detection and laser pulse, photon timestamps can be re-synchronized to the periodic laser source and a histogram free from pile-up distortion can be captured.

%\newpage
%{\small
%\bibliographystyle{splncs04}
%\bibliography{HistoVision}
%}
%\end{document}
